# Supplementary material for: Formation and dynamics of van der Waals molecules in buffer-gas traps
Source: arXiv:1104.4973 source file (2011-04-26)
Supplement: Supplementary file 1 [file line-appendix.pdf]

## A Spectral line intensities

In the adiabatic approximation, the Hamiltonian of the ground electronic state can be written as

$$\hat{H}_g = -\frac{1}{2\mu r}\frac{\partial^2}{\partial r^2}r + \frac{\hat{N}^2}{2\mu R^2} + V(r), \tag{1}$$

where $r$ is the interatomic distance, $N$ is the rotational angular momentum, $\mu$ is the reduced mass, and $V(r)$ is the interaction potential. For simplicity, we omit the hyperfine interactions, the spin-rotation interaction, and consider the case of zero external magnetic field. We use Hund's case (a) basis functions

$$|JM\Omega\rangle|\Lambda\Sigma\rangle \tag{2}$$

where $J$ is the total angular momentum $\hat{J} = \hat{N} + \hat{L} + \hat{S}$, where $\hat{L}$ is the electronic orbital angular momentum and $\Sigma$ is the electron spin. $\Lambda$ and $\Sigma$ are the projections of $\hat{L}$ and $\hat{S}$ onto the internuclear axis, and $\Omega = \Lambda + \Sigma$. For $^2\Sigma$ electronic states, $\Lambda = 0$ and hence $\Omega = \Sigma$. The most important term in Eqn. (1) is the rotational kinetic energy, which can be written in Hund's case (a) as

$$B_e(\hat{J} - \hat{S})^2 = B_e(\hat{J}^2 + \hat{S}^2 - 2\hat{J}_z\hat{S}_z - \hat{J}_+\hat{S}_+ - \hat{J}_+\hat{S}_-) \tag{3}$$

The cross terms $\hat{J}_\mp\hat{S}_\pm$ couple the states with different $\Sigma$, but $J$ remains a good quantum number. The eigenfunctions of the ground-state Hamiltonian can therefore be written as linear combinations of basis functions of Eqn. (2) with the same $J$ but different $\Omega$ ($\Omega$ and $\Sigma$ can be used interchangeably here)

$$|nJM\rangle = \sum_{\Omega=-1/2}^{1/2} a_{J\Omega}|JM\Omega\rangle|\Lambda = 0, \Omega\rangle \tag{4}$$

Eqn. (3) contains cross terms, which lead to large (of order $B_e$) off-diagonal matrix elements of $\hat{H}_g$. Therefore, Hund's case (a) scheme is not optimal for describing rotational dynamics of $^2\Sigma$ molecules. In fact, all $^2\Sigma$ molecules fall in Hund's case (b) category since the absence of the first-order spin-orbit interaction makes $N$ a good quantum number. Hund's case (b) rotational basis functions have the form

$$|NJS\rangle, \tag{5}$$

where $N$ is the rotational angular momentum. In the absence of the spin-rotation interaction (such as in our case), the Hamiltonian in basis (2) has

only diagonal matrix elements, which are given by

$$\langle NJS|\hat{H}_g|NJS\rangle = -\frac{1}{2\mu r}\frac{\partial^2}{\partial r^2}r + \frac{N(N+1)}{2\mu R^2} + V(r), \tag{6}$$

where $N$ is an integer number. Note that $\Sigma$ is not defined in Hund's case (b). Numerical solution of Eqn. (6) gives ro-vibrational energies $\epsilon_{vJ}$ and wave functions $\chi_{vJ}(r)$. Since these energies only depend on $r$, we can use them to augment Eqn. (2). As a result, the full ro-vibrational eigenfunction for the ground electronic state of AgHe takes the form

$$\chi_{vJ}(r)|nJ\rangle = \chi_{vJ}(r)\sum_{\Omega=-1/2}^{1/2} a_{J\Omega}|JM\Omega\rangle|\Lambda = 0, \Omega\rangle \tag{7}$$

The Hamiltonian for the excited $^2\Pi_{3/2}$ state of AgHe may be written as

$$\hat{H}_e = -\frac{1}{2\mu r}\frac{\partial^2}{\partial r^2}r + \frac{\hat{N}^2}{2\mu R^2} + V(r) + H_{\mathrm{SO}}, \tag{8}$$

where the additional term $\hat{H}_{\mathrm{SO}}$ represents the spin-orbit interaction

$$\hat{H}_{\mathrm{SO}} = A_{\mathrm{SO}}\hat{L}\cdot\hat{S} = \frac{A_{\mathrm{SO}}}{2}\left[\hat{J}_a^2 - \hat{L}^2 - \hat{S}^2\right], \tag{9}$$

where $\hat{J}_a = \hat{L}+\hat{S}$ is the total angular momentum of the Ag atom exclusive of nuclear spin, and $A_{\mathrm{SO}}$ is related to the fine-structure splitting of the $^2P$ term. Since only the $^2\Pi_{3/2}$ electronic state of AgHe has a non-negligible Franck-Condon overlap with the ground state, we have $J_a = \frac{3}{2}$. The rotational energy can be written as

$$B_e(\hat{J} - \hat{J}_a)^2 = B_e(\hat{J}^2 + \hat{J}_a^2 - 2\hat{J}_z\hat{J}_{az} - \hat{J}_+\hat{J}_{a-} - \hat{J}_-\hat{J}_{a+}) \tag{10}$$

The cross terms change the value of $\Omega$ - the projection of $J$ and $J_a$ onto the internuclear axis. In our case, $\Omega = \frac{3}{2}$. Fig. 1 shows that the other electronic state of $\Omega = 1/2$ symmetry is far apart in energy, so the cross terms have a negligible effect. The Hamiltonian of Eqn. (8) is diagonal in Hund's case (c) basis [1, 2]

$$|JM\Omega\rangle|J_a\Omega\rangle, \tag{11}$$

where, as before, $\hat{J} = \hat{N}+\hat{J}_a$ is the total angular momentum with space-fixed and molecule-fixed projections $M$ and $\Omega$. Note that when $J_a = S$ (ground electronic state), Hund's case (a) with $\Lambda = 0$ is recovered. For evaluating

transition probabilities, it is essential that the same representation be used for both ground and excited states. This is the main reason why we used case (a) basis for the ground electronic state, despite the fact that Hund's case (b) scheme offers more meaningful quantum numbers.

The effective Hamiltonian for Hund's case (c) takes the form [1]

$$\langle JM\Omega|\langle J\Omega|\hat{H}_g|JM\Omega\rangle|J_a\Omega\rangle = -\frac{1}{2\mu r}\frac{\partial^2}{\partial r^2}r + \frac{J(J+1)+J_a(J_a+1)-2\Omega^2}{2\mu R^2} + V_\Omega(r), \quad (12)$$

The energy levels $\epsilon_{vJJ_a\Omega}$ and wave functions $\chi_{vJJ_a\Omega}(r)$ are obtained by quantizing the Hamiltonian of Eqn. (12) using the potential energy curve for the $^2\Pi_{3/2}$ electronic state. The total ro-vibrational wave function may be written

$$\chi_{vJJ_a\Omega}(r)|JM\Omega\rangle|J_a\Omega\rangle. \quad (13)$$

The probabilities for electric dipole transitions are given by [2, 3]

$$P(nvJ \to v'J'J'_a\Omega') \propto \sum_{M,M'} |\langle nJM|\langle\chi_{vJ}(r)|\mu_Z(1,0)|\chi_{vJJ_a\Omega}(r)\rangle|JM\Omega\rangle|J_a\Omega\rangle|^2, \quad (14)$$

where $\mu_Z(1,0)$ is the space-fixed transition dipole moment, which we transform to the molecule-fixed frame

$$\mu_Z(1,0) = \sum_q D^{1\star}_{0q}\mu(1,q), \quad (15)$$

where $q$ denotes the molecule-frame component of $\mu$ and $D^{1\star}_{0q}$ are the Wigner $D$-functions. Substituting Eqn. (15) into Eqn. (14), factoring out the Franck-Condon overlap, and evaluating the matrix element of three $D$-functions [3], we find

$$P(nvJ \to v'J'J'_a\Omega') \propto [(2J'+1)(2J+1)]\langle\chi_{v'J'J'_a\Omega'}(r)|\chi_{vJ}(r)\rangle^2 \times \sum_{M,M'}\left|\sum_{\Omega=-1/2}^{1/2} a_{J\Omega}\begin{pmatrix} J' & 1 & J \\ M' & 0 & -M\end{pmatrix}\begin{pmatrix} J' & 1 & J \\ \Omega' & \Omega-\Omega' & -\Omega\end{pmatrix} \times \langle J'_a\Omega'|\mu(1,\Omega'-\Omega)|\Lambda=0,\Omega\rangle\right|^2. \quad (16)$$

The sum over $M$ and $M'$ can be evaluated using the orthogonality properties of 3-$j$ symbols [3] to yield

$$P(nvJ \to v'J'J_a'\Omega') \propto [(2J'+1)(2J+1)]\langle \chi_{v'J'J_a'\Omega'}(r)|\chi_{vJ}(r)\rangle^2$$
$$\times \left| \sum_{\Omega=-1/2}^{1/2} a_{J\Omega} \begin{pmatrix} J' & 1 & J \\ \Omega' & \Omega-\Omega' & -\Omega \end{pmatrix} \langle J_a'\Omega'|\mu(1,\Omega'-\Omega)|\Lambda=0,\Omega\rangle \right|^2. \quad (17)$$

Since $\Omega' = \frac{3}{2}$, the $\Omega = -1/2$ term in the sum in Eqn. (17) gives $\Omega' - \Omega = 2$ which is forbidden because the dipole moment tensor has rank 1. Therefore, the sum in Eqn. (17) collapses to a single term. In the absence of the spin-rotation interaction, the coefficients $a_{J\Omega}$ do not depend on $J$ and can therefore be omitted. As a result of these simplifications, we obtain

$$P(nvJ \to v'J'J_a'\Omega' = \tfrac{3}{2}) \propto [(2J'+1)(2J+1)]\langle \chi_{v'J'J_a'\Omega'}(r)|\chi_{vJ}(r)\rangle^2$$
$$\times \left| \begin{pmatrix} J' & 1 & J \\ \Omega' & \Omega-\Omega' & -\Omega \end{pmatrix} \langle J_a'\Omega'|\mu(1,\Omega'-\Omega)|\Lambda=0,\Omega\rangle \right|^2. \quad (18)$$

Finally, we assume that the transition dipole matrix element of AgHe is the same as that of Ag.

# References


[1] H. Lefebvre-Brion and R. W. Field, *The spectra and Dynamics of Diatomic Molecules* (Elsevier, Amsterdam, 2004), p. 124.

[2] Y. Zhao, I. Yourshaw, G. Reiser, C. C. Arnold, and D. M. Neumark, J. Chem. Phys. **101**, 6538 (1994).

[3] R. N. Zare, *Angular momentum* (Wiley, NY, 1988).
